# Supplementary material for: The Photographer Eye: Teaching Multimodal Large Language Models to Understand Image Aesthetics like Photographers
Source: arXiv:2509.18582 source file (2025-10-22)
Supplement: Supplementary file 2 [file appendix.tex]

Hi
